# Supplementary material for: Indoor positioning systems: Smart fusion of a variety of sensor readings
Source: arXiv:2105.05438 source file (2021-05-12)
Supplement: Supplementary file 1 [file appendix.tex]

\section{NN parameters}
Appendix
